# Supplementary material for: Bridging the gap between natural user expression with complex automation programming in smart homes
Source: arXiv:2408.12687 source file (2024-08-22)
Supplement: Supplementary file 1 [file appendix.tex]

\appendix

\begin{table}
  \caption{Interaction Challenges of Smart Home Automation}
  \label{tab:freq}
  \begin{tabular}{ccl}
    \toprule
    Challenges& Definitions \& Descriptions & Resolution\\
    \midrule
     \multirow{Feasibility and usability} & Inflexibility to complex situations and human uncertainty & For Swedish names\\~&Reliability, frequent system failures&For Swedish name \\~&Multi-user conflicts and tensions&For Swedish name \\
   \multirow{Manageability}& Poor in manageability in technical expertise, long-term testing [hacking]& Common in math\\~& System Management&For Swedish name \\

    \multirow{End-user Programming} & Match users‘ intention [IIP]  & Used in business\\~&Natrural and high-semantic Programming& Used in business\\~&Complex rules& Used in business\\
   Privacy and Security & Privacy & Unexplained usage\\
   Value& Perceivable, Acceptance& Unexplained usage\\
   Sharing&Sharing,community& Unexplained usage\\
   Cost of Appropriation& cost,energy& Unexplained usage\\
  \bottomrule
\end{tabular}
\end{table}
